# Supplementary material for: Joint Edge-Model Sparse Learning is Provably Efficient for Graph Neural Networks
Source: arXiv:2302.02922 source file (2023-02-06)
Supplement: Supplementary file 1 [file appendix_copy.tex]

\section{Overview of the techniques}\label{sec: max-pooling}
The main idea of the proof is to describe the updates of $\bfW$, and a similar result for $\bfU$ can be derived using the same method. 
% For the convenience of presentation, we define random variables $\bfx^+$ and $\bfx^-$ such that $(\bfx^+ , +1 ) \sim (\mathcal{X},\mathcal{Y})$ and $(\bfx^- , -1 ) \sim (\mathcal{X},\mathcal{Y})$. 
% Recall that 
% \begin{equation}\label{eqn: defi_x}
%     \bfx = \begin{bmatrix} \bfx_1^\top & \bfx_2^\top & \cdots & \bfx_M^\top \end{bmatrix}^\top.
% \end{equation}
% W.L.O.G., we assume $\bfx^+_{1} = \bfp_+$ and $\bfx^-_{1} =\bfp_-$. 
Recall that at iteration $t$, the aggregator function for node $v$ is written as
\begin{equation}
    \text{AGG}(\bfX_{\mathcal{N}_s^{(t)}(v)},\bfw_k^{(t)}) = \max_{n\in \mathcal{N}(v)}~\phi(\vm{\bfw_k^{(t)}}{\bfx_n}).
\end{equation}
Then,  at iteration $t$,
we define the 
% identification function $I: \mathbb{R}\rightarrow \{0, 1 \}$ as
% \begin{equation}\label{eqn: identification}
%     =
%     \begin{cases}
%         1, \quad \text{if}\quad y\cdot g(\bfW,\bfV;\bfx)<1 \\
%         0, \quad \text{if}\quad y\cdot g(\bfW,\bfV;\bfx)>1
%     \end{cases},
% \end{equation}
% and 
pattern function $\mathcal{M}^{(t)}: \mathcal{V} \rightarrow \mathcal{P}\bigcup\{\bfzero\}$ as
\begin{equation}\label{eqn: pattern_function}
    \mathcal{M}^{(t)}(v;\bfw) = \begin{cases}
        \mathbf{0}, \quad \text{if} \quad \displaystyle\max_{n\in\ns[t](v)} \phi( \vm{\bfw}{\bfx_{n}} )\le 0\\
       \displaystyle\argmax_{\{\bfx_n \mid n\in\ns[t](v)\}} \phi( \vm{\bfw}{\bfx_{n}} ), \quad \text{otherwise}
    \end{cases}.
\end{equation}

\textbf{Lucky Neuron.} We call a neuron is the \textit{lucky neuron} if and only if  its weights vector satisfies
\begin{equation}\label{defi:lucky_filter}
\begin{gathered}
    \mathcal{M}{(v;\bfw_k)} = \bfp_+ \quad \text{for any} \quad v\in\mathcal{V}
\end{gathered}
\end{equation}
and 
\begin{equation}\label{defi:lucky_filter_v}
        \mathcal{M}{(v;\bfu_k)} = \bfp_- \quad \text{for any} \quad v\in\mathcal{V}
\end{equation}
for $\{\bfw_k \}_{k=1}^K$ and $\{\bfu_k\}_{k=1}^K$, respectively.

For simplification, we will not consider the neuron that $\max_{\bfp \in \mathcal{P}}\vm{\bfw_k^{(0)}}{\bfp}<0$ because such neuron will not be updated or make any contribution in $g(\bfW,\bfU;v)$.

% \subsection{}
\textbf{Gradient of the \textit{lucky neuron} and \textit{unlucky neuron}.} The gradient of $\hat{f}$ is
\begin{equation}
\begin{split}
    \frac{\partial \hat{f}^{(t)}_{\Omega}}{\partial \bfw_k^{(t)}} 
    =& -\frac{1}{|\Omega|} \sum_{v\in\Omega} ~y_v\cdot \frac{\partial g(\bfW^{(t)},\bfU^{(t)};\bfX_{\ns[t](v)})}{\partial \bfw_k^{(t)}}\\
    =& - \frac{1}{|\Omega_+|} \sum_{v\in\Omega_+} ~\frac{\partial g(\bfW^{(t)},\bfU^{(t)};\bfX_{\ns[t](v)})}{\partial \bfw_k^{(t)}} 
    + \frac{1}{|\Omega_-|} \sum_{v\in\Omega_-} ~\frac{\partial g(\bfW^{(t)},\bfU^{(t)};\bfX_{\ns[t](v)})}{\partial \bfw_k^{(t)}}
\end{split}
\end{equation}
% and the update rule of $\{\bfw_k^{(t)}\}_{t=1}^T$ is 
% \begin{equation}\label{eqn: update_g}
% \begin{split}
%     \bfw_k^{(t+1)} 
%     =& \bfw_k^{(t)} -\eta\frac{\partial \hat{f}}{\partial \bfw_k}(\bfw_k^{(t)})\\
%     =& \bfw_k^{(t)} + \eta\cdot\mathbb{E}_{\bfx^+ \in \mathcal{D}_+}\frac{\partial g(\bfW,\bfV;\bfx^+)}{\partial \bfw_k} - \eta\cdot \mathbb{E}_{\bfx^- \in \mathcal{D}_-}\frac{\partial g(\bfW,\bfV;\bfx^-)}{\partial \bfw_k}.
% \end{split}
% \end{equation}
%  For an input $\bfx \in \mathcal{X}$, let us define $\mathcal{M}(\bfx) \in \{\bfx_m \}_{m=1}^M$ be the vector such that 
According to the definition of $\mathcal{M}^{(t)}$ in \eqref{eqn: pattern_function}, it is easy to verify that 
 \begin{equation}
     \frac{\partial g(\bfW^{(t)},\bfU^{(t)};\bfX_{\ns[t](v)})}{\partial \bfw_k^{(t)}} = \mathcal{M}^{(t)}(v;\bfw_k^{(t)}),
 \end{equation}
and the update of $\bfw_k$ is
\begin{equation}\label{eqn: update_g_2}
\begin{split}
    \bfw_k^{(t+1)} 
    = \bfw_k^{(t)} + \eta\cdot\mathbb{E}_{v \in \Omega_+}\mathcal{M}^{(t)}(v;\bfw_k^{(t)}) - \eta\cdot \mathbb{E}_{v\in \Omega_-}\mathcal{M}^{(t)}(v;\bfw_k^{(t)}).
\end{split}
\end{equation}

\subsection{Sketchy of the proof}
Note that $\bfp_+$ only exists in the neighbors of node $v$ with positive label, $\bfp_-$ only exists in the neighbors of node $v$ with negative label, and non-discriminative patterns $\mathcal{P}$ are distributed in $\bfx_+$ and $\bfx_-$ identically. For \textit{lucky neuron}, $\mathcal{M}(v)$ is always $\bfp_+$ for $v\in\Omega_+$, and $\mathcal{M}(v)$ is always orthogonal to $\bfp_+$ for $v\in\Omega_-$. Therefore, the weights of the lucky neuron will strictly increase in the direction of $\bfp^+$. For \textit{unlucky neuron}, because non-discriminative patterns are identically distributed in $\bfx$ and independent of $y$. Therefore, the gradient generated from $\Omega_+$ and $\Omega_-$ are similar, and the overall gradient is in the order of $\sqrt{{(1+r^2)}/{N}}$ because of the offsets between $\Omega_+$ and $\Omega_-$.

In the following contents, we will provide a comprehensive proof, and Figure \ref{fig: fliter} depicts the major findings about the update of neuron weights. 
\begin{figure}[h]
     \centering
     \begin{subfigure}[b]{0.40\textwidth}
         \centering
         \includegraphics[width=\textwidth]{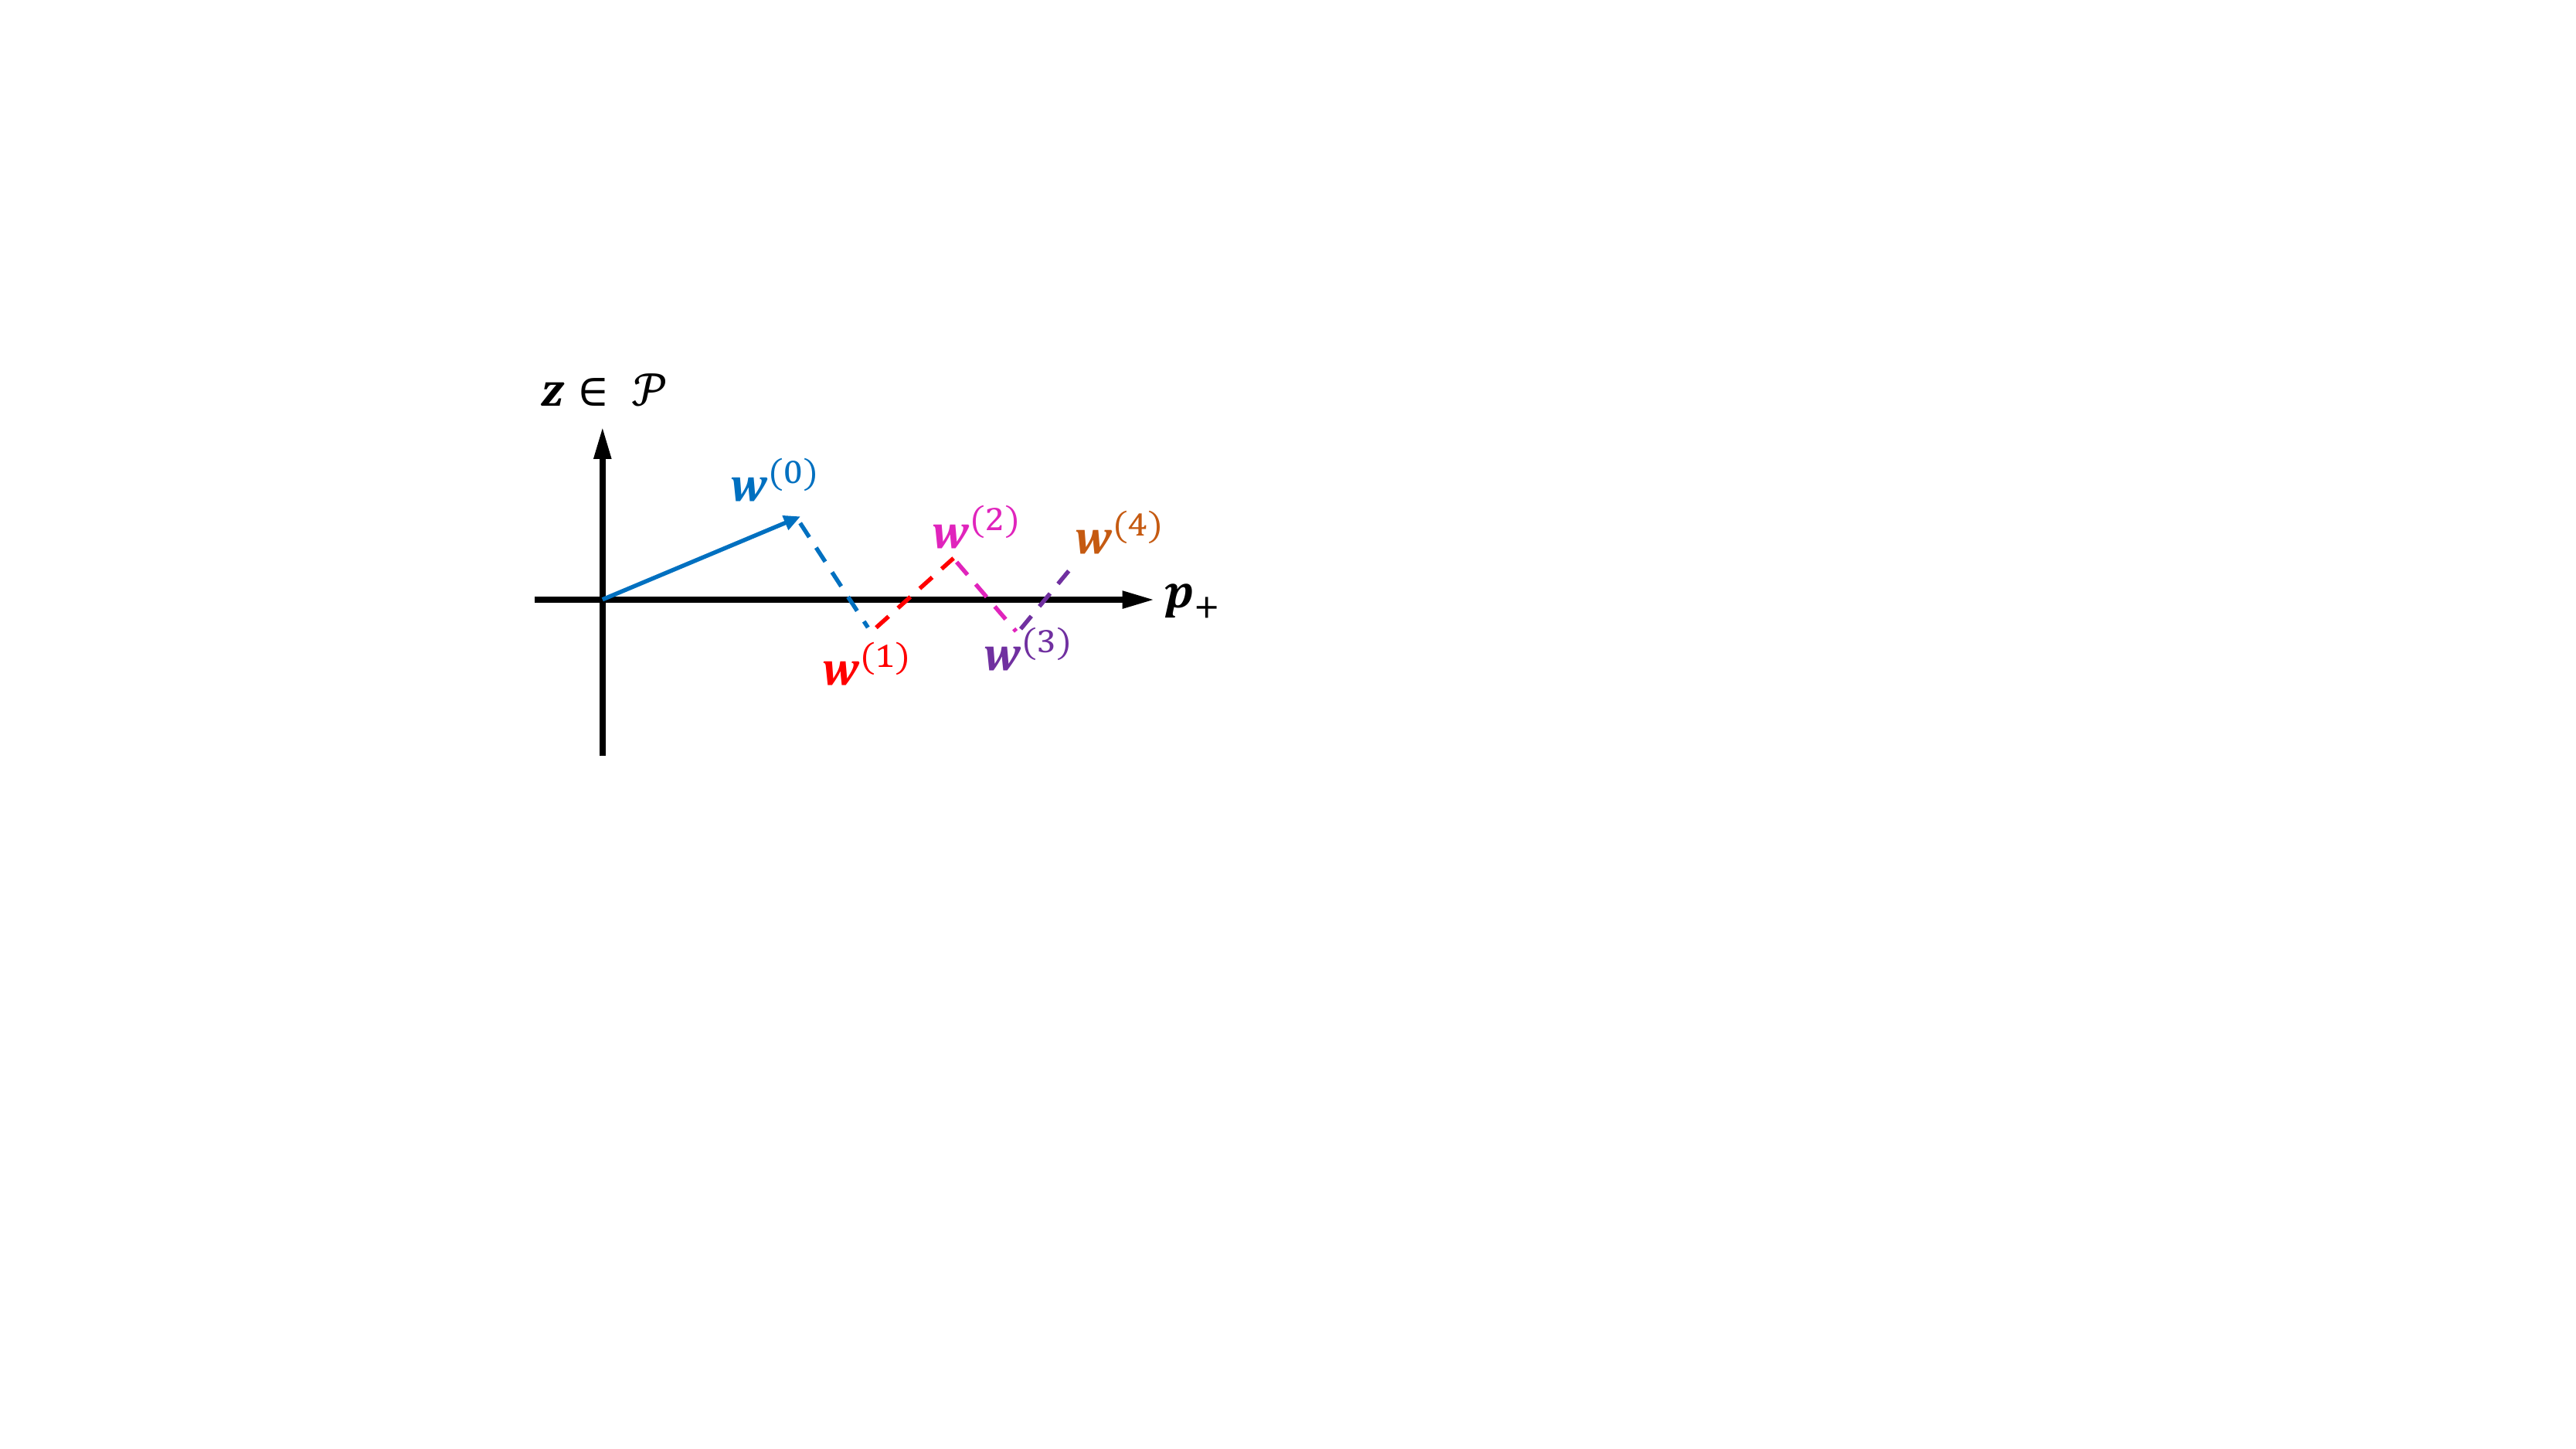}
         \caption{}
         \label{fig: lucky}
     \end{subfigure}
     \hfill
     \begin{subfigure}[b]{0.40\textwidth}
         \centering
         \includegraphics[width=\textwidth]{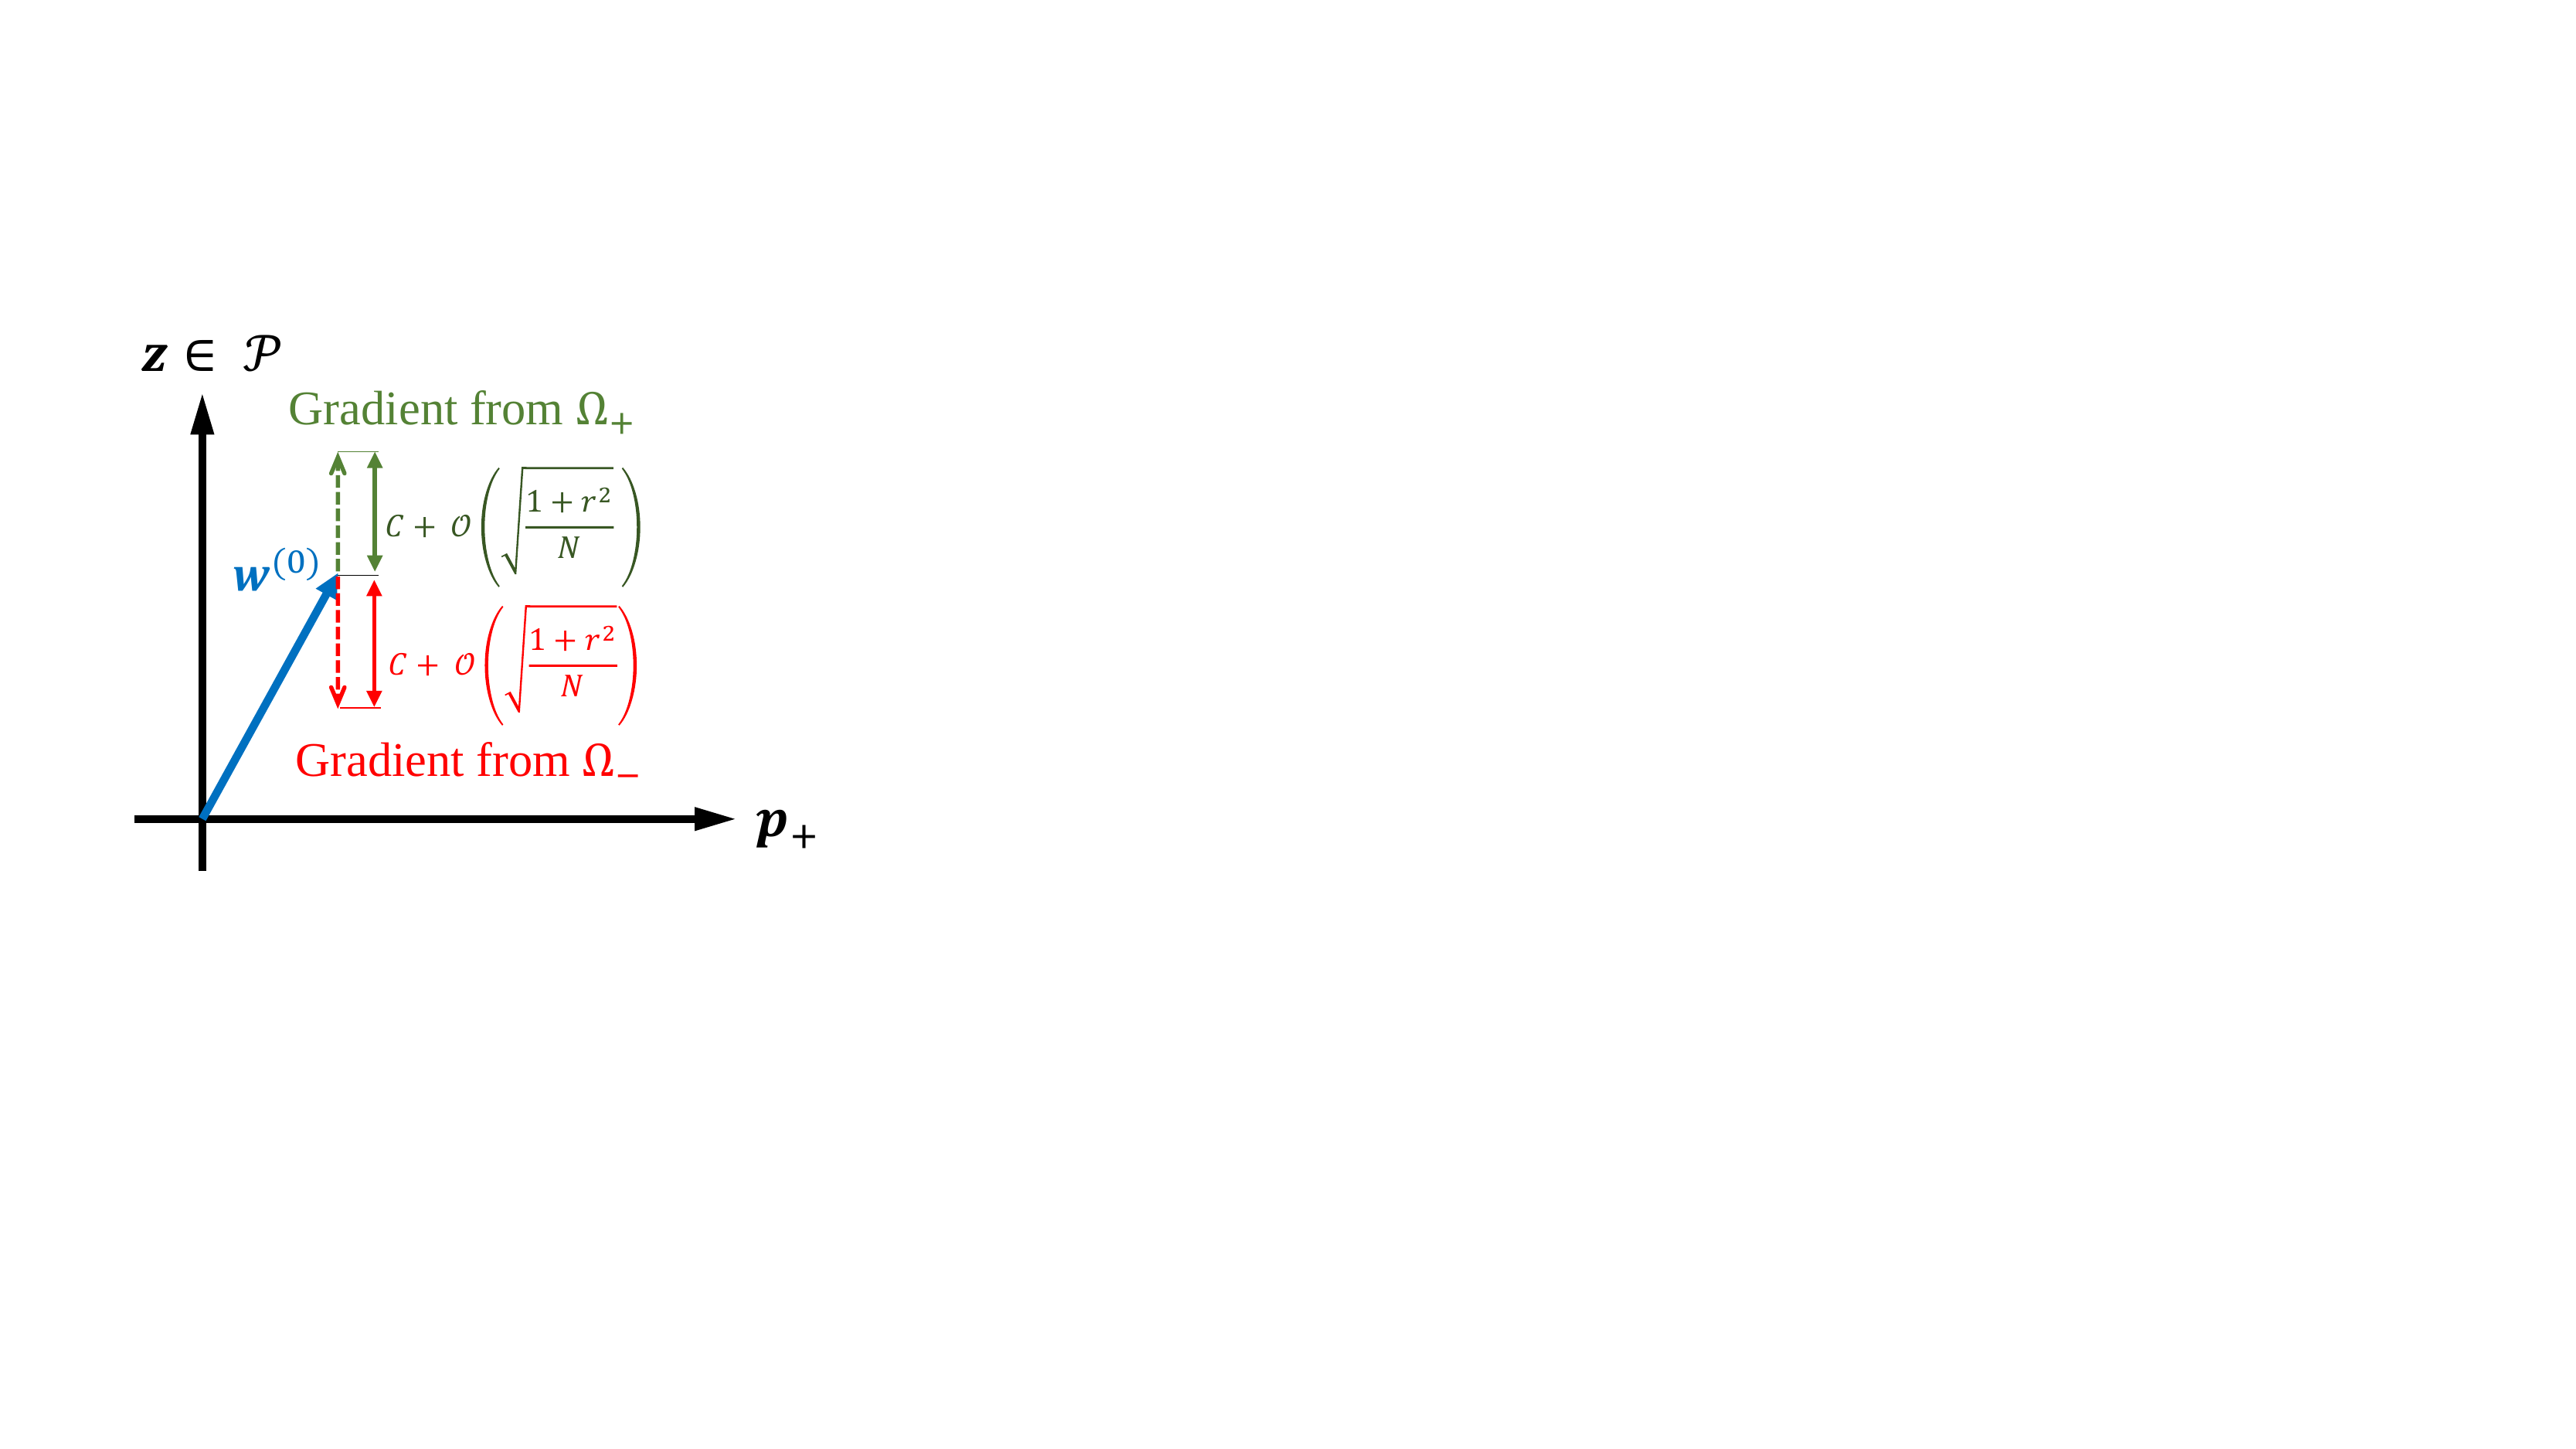}
         \caption{}
         \label{fig: unlucky}
     \end{subfigure}
        \caption{Illustration of iterations $\{\bfw^{(t)}\}_{t=1}^T$: (a) \textit{lucky neuron}, and (b) \textit{unlucky neuron}.}
        \label{fig: fliter}
\end{figure}

\section{Useful Lemmas}
\begin{lemma}\label{Lemma: number_of_lucky_neuron}
With high probability (W.H.P.), $\Theta(\frac{1}{L})$ fraction of neurons are  the \textit{lucky neuron}. 
% \begin{figure}[h]
%     \centering
%     \includegraphics[width = 0.35\linewidth]{Figure/L.pdf}
%     \caption{Probability of lucky filters when $L$ varies.}
%     \label{fig: lucky_filter}
% \end{figure}
\end{lemma}
\begin{lemma}\label{Lemma: update_lucky_neuron}
    For lucky neuron $\bfw_k^{(0)}$, we have
    
    1. $\vm{\bfw_k^{(t+1)}}{\bfp_+} \ge \vm{\bfw_k^{(t)}}{\bfp_+}  + \eta\|\bfp_+\|_2$;
    
    2. $-\eta\le \vm{\bfw_k^{(t)}}{\bfz} \le \vm{\bfw_k^{(0)}}{\bfz}$ for any $\bfz \in \mathcal{P}/\bfp_+$.
\end{lemma}
\begin{lemma}\label{Lemma: update_unlucky_neuron}
    For unlucky neuron $\bfw_k^{(0)}$, we have
    
    1. $\vm{\bfw_k^{(t+1)}}{\bfp_+} \ge \vm{\bfw_k^{(t)}}{\bfp_+}$;
    
    2. $-\eta\le \vm{\bfw_k^{(t)}}{\bfp_-} \le \vm{\bfw_k^{(0)}}{\bfp_-}$ for $t\ge0$;
    
    3. $\big|\vm{\bfw_k^{(t+1)}}{\bfz}-\vm{\bfw_k^{(t)}}{\bfz}\big| \le  \eta\cdot \sqrt{\frac{\log q}{N}}\cdot\|\bfz\|^2$ for any $\bfz \in \mathcal{P}_s$.
\end{lemma}
\begin{lemma}\label{Lemma: number_of_lucky_filter}
    Let $\mathcal{U}(t)$ be the set of the \textit{lucky neuron} at $t$-th iteration such that
    \begin{equation}
        \mathcal{U}(t) = \{ k \mid \mathcal{M}^{(t)}(v;\bfw_k^{(t)}) = \bfp_+ \quad \text{for any}\quad  v\in \mathcal{V} \}. 
    \end{equation}
    Then, we have 
    \begin{equation}
        \mathcal{U}(0)\subseteq \mathcal{U}(t).
    \end{equation}
\end{lemma}


\section{Proof of Main Theorem}

\begin{proof}[Proof of Theorem \ref{Thm:major_thm}]
    For any point $\bfx\in\mathcal{X}$ with label $y=1$, we have
    \begin{equation}
    \begin{split}
        & g(\bfW^{(t)},\bfU^{(t)};\bfv) \\
        = & \sum_{k=1}^K \max_{n\in\mathcal{N}(v)}~\phi\big(\vm{\bfw_k^{(t)}}{\bfx_n}\big) - \sum_{k=1}^K \max_{n\in\mathcal{N}(v)}~\phi\big(\vm{\bfu_k^{(t)}}{\bfx_n}\big)\\
        = & \sum_{k\in\mathcal{U}(t)} \vm{\bfw_k^{(t)}}{\bfp_+} + \sum_{k\in[K]/\mathcal{U}(t)}\max_{n\in\mathcal{N}(v)}~ \phi\big(\vm{\bfw_k^{(t)}}{\bfx_n}\big) -\sum_{k=1}^K \max_{n\in\mathcal{N}(v)}~\phi\big(\vm{\bfu_k^{(t)}}{\bfx_n}\big)\\
        \ge &\sum_{k\in\mathcal{U}(t)} \vm{\bfw_k^{(t)}}{\bfp_+} -\sum_{k=1}^{K} \max_{n\in\mathcal{N}(v)}~\phi\big(\vm{\bfu_k^{(t)}}{\bfx_n}\big),    
    \end{split} 
    \end{equation}
    where $\mathcal{U}(t)$ is the set of \textit{lucky filters} with respect to weights $\{\bfw_k\}_{k=1}^K$.
    
    Then, from Lemma \ref{Lemma: number_of_lucky_neuron}, Lemma \ref{Lemma: update_lucky_neuron}, and Lemma \ref{Lemma: number_of_lucky_filter}, we have
    \begin{equation}\label{eqn: update_w}
        \begin{split}
        \sum_{k\in\mathcal{U}(t)} \vm{\bfw_k^{(t)}}{\bfp_+} 
        \ge& |\mathcal{U}_t|\cdot \eta \cdot \|\bfp_+\|^2t\\
        \ge& |\mathcal{U}_0|\cdot \eta \cdot \|\bfp_+\|^2t\\
        \ge& \frac{K}{L}\cdot \eta \cdot \|\bfp_+\|^2t.
        \end{split} 
    \end{equation}
    From Lemma \ref{Lemma: update_unlucky_neuron}, we have
    \begin{equation}\label{eqn: update_v}
        \begin{split}
            \sum_{k=1}^K \max_{n\in\mathcal{N}(v)}~\phi\big(\vm{\bfu_k^{(t)}}{\bfx_n}\big)
            \le & K\eta\cdot \sqrt{\frac{d \log q}{N}}\cdot\|\bfp_+\|^2\\
            \le & \varepsilon\cdot \frac{K}{L}\cdot \eta \|\bfp_+\|^2t,
        \end{split}
    \end{equation}
    where the last inequality comes from the assumption that $N>\varepsilon^{-2} L^2 d\log q$.
    
    Combining \eqref{eqn: update_w} and \eqref{eqn: update_v}, we have 
    \begin{equation}\label{eqn:update_x+}
        g(\bfW^{(t)},\bfU^{(t)};v) \ge (1-\varepsilon)\frac{K\eta}{L}\|\bfp_+\|^2 t.
    \end{equation}
    Therefore, when $t>\frac{L}{(1-\varepsilon)K\eta}$, we have $g(\bfW^{(t)},\bfU^{(t)};v)>1$. Similar to the proof of \eqref{eqn:update_x+}, we can show that $g(\bfW^{(t)},\bfU^{(t)};v)<-1$
    for any $v\in\mathcal{V}$ with label $y=-1$.
    
    In conclusion, the generalization function \eqref{eqn: generalization_error} achieves zero when $t>\frac{L}{(1-\varepsilon)K\eta}$.
\end{proof}

\section{Proof of Useful Lemmas}

\subsection{Proof of Lemma \ref{Lemma: number_of_lucky_neuron}}
\begin{proof}[Proof of Lemma \ref{Lemma: number_of_lucky_neuron}]
For a random generated weights $\bfw_k$, let us define the random variable $i_k$ such that
    \begin{equation}
        i_k = \begin{cases}
            1, \quad \text{if  $\bfw_k$ is the \textit{lucky filter}}\\
            0, \quad \text{otherwise}
        \end{cases}.
    \end{equation}
    From the contents below, we know $i_k$ belongs to Bernoulli distribution with probability $1/L$. By Hoeffding's inequality, we know that
    \begin{equation}
    \frac{1}{L} - \sqrt{\frac{C\log q}{K}} \le   \frac{1}{K}\sum_{k=1}^{K}i_k \le \frac{1}{L} + \sqrt{\frac{C\log q}{K}}
    \end{equation}
    with probability at least $q^{-C}$.
    Let $K = \Omega(L^2\log q)$, we have $\frac{1}{K}\sum_{k=1}^{K}i_k = \Theta(\frac{1}{L})$.
   
   Let $\theta_1$ be the angle between $\bfp_+$ and the initial weights $\bfw$. Let $\{\theta_\ell \}_{\ell=2}^L$ be the angles between $\bfp_-$ and $\bfp \in \mathcal{P}_s$. Then, it is easy to verify that $\{ \theta_\ell\}_{\ell=1}^L$ belongs to the uniform distribution on the interval $[ 0 , 2\pi]$. Because $\bfp \in \mathcal{P}$ are orthogonal to each other. Then, $\vm{\bfw}{\bfp}$ with $\bfp\in \mathcal{P}$ are independent with each other given $\bfw$ belongs to Gaussian distribution. 
   It is equivalent to say that $\{\theta_\ell \}_{\ell =1}^L$ are independent with each other. Consider the noise level $\sigma$ is significantly smaller than $\|\bfp\|_2$, then the probability of lucky neuron can be bounded as 
    \begin{equation}
        \text{Prob}\Big( \theta_1 +\Delta\theta \le \theta_i - \Delta \theta \le 2\pi , \quad 2\le i \le L \Big), 
    \end{equation}
    where $\Delta \theta \simeq \frac{\sigma}{\|\bfp\|_2}$.
    Then, we have
    \begin{equation}
    \begin{split}
          &\text{Prob} \Big(  \theta_1 +\Delta\theta \le \theta_\ell - \Delta \theta \le 2\pi , \quad 2\le \ell \le L \Big)\\
        = & \prod_{\ell =1}^L \text{Prob}\Big( \theta_1 +\Delta\theta \le \theta_\ell - \Delta \theta \le 2\pi \Big)\\
        = & \bigg(\frac{2\pi -\theta_1 - \Delta \theta}{2\pi}\bigg)^{L-1}.
    \end{split}
    \end{equation}
    Next, we can bound the probability as
    \begin{equation}
    \begin{split}
          \text{Prob} (  \bfw \text{ is the lucky neuron} )
        = & \int_{0}^{2\pi} \frac{1}{2\pi} \cdot \bigg(\frac{2\pi -\theta_1 - \Delta \theta}{2\pi}\bigg)^{L-1} d\theta_1\\
        \simeq & \frac{1}{L} \cdot \bigg(\frac{2\pi - 2 \Delta \theta}{2\pi}\bigg)^L\\
        \simeq & \frac{1}{L} \cdot \bigg(1 - \frac{ L\sigma}{\pi\|\bfp\|_2}\bigg).
    \end{split}    
    \end{equation}
    
    
%   Given $\bfp_+$, we randomly select $L$ number of vectors $\{\bfp_\ell\}_{\ell =1}^L$ such that are orthogonal to $\bfp_+$. Randomly choose a vector $\bfw$, with probability at least $\frac{1}{L}$ such that $\vm{\bfw}{\bfp_+}\ge \max_{\ell}\vm{\bfw}{\bfp_\ell}$.

%     Let $\theta$ denote the angle between $\bfp_+$ and $\bfw$, and it is easy to verify that $\theta$ belongs to the uniform distribution on the interval $[0, 2\pi]$. Then, we want to know that probability that 
%     \begin{equation}
%     \begin{split}
%         &\text{Prob}\Big(\vm{\bfw}{\bfp_1}\le \cos\theta, \vm{\bfw}{\bfp_2}\le \cos\theta, \cdots, \vm{\bfw}{\bfp_L}\le \cos\theta\Big)\\
%     \end{split}
%     \end{equation}
%     Because $\bfp_+$ are orthogonal to $\bfp_\ell$, $\vm{\bfw}{\bfp_+}$ or $\theta$ is independent with $\vm{\bfw}{\bfp_\ell}$ for $\ell \in [L]$. Therefore, we have 
%     \begin{equation}
%     \begin{split}
%             &\text{Prob}\Big(\vm{\bfw}{\bfp_1}\le \cos\theta, \vm{\bfw}{\bfp_2}\le \cos\theta, \cdots, \vm{\bfw}{\bfp_L}\le \cos\theta\Big)\\
%         = & \text{Prob}\Big(\vm{\bfw}{\bfp_1}\le \cos\theta\Big) \cdot \text{Prob}\Big(\vm{\bfw}{\bfp_2}\le \cos\theta\Big) \cdots \text{Prob}\Big(\vm{\bfw}{\bfp_L}\le \cos\theta\Big)\\
%         = & \Big(\frac{\theta}{2\pi}\Big)^L.
%     \end{split}
%     \end{equation}
%     Then, we have
%     \begin{equation}
%     \begin{split}
%             & \text{Prob}\big(\vm{\bfw}{\bfp_+}\ge \max_{\ell}\vm{\bfw}{\bfp_\ell}\big)\\
%         = & \int_{0}^{2\pi} \frac{1}{2\pi}\Big(\frac{\theta}{2\pi}\Big)^L d\theta\\
%         = & \frac{1}{L+1}
%     \end{split}
%     \end{equation}
\end{proof}

\subsection{Proof of Lemma \ref{Lemma: update_lucky_neuron}}
\begin{proof}[Proof of Lemma \ref{Lemma: update_lucky_neuron}]
For any $v \in\Omega_+$ and a lucky neuron with weights $\bfw_k^{(t)}$, we have
\begin{equation}
\begin{gathered}
    \max_{n\in\ns[t](v)} \phi(\vm{\bfw_k^{(t)}}{\bfx_n}) = \phi(\vm{\bfw_k^{(t)}}{\bfp_+}),\\
    \text{and}\qquad  \mathcal{M}^{(t)}(v;\bfw_k^{(t)}) = \bfp_+.
\end{gathered}
\end{equation}
Then, the gradient is calculated as
\begin{equation}\label{eqn: lemma1_1_+}
    \frac{\partial g(\bfW^{(t)},\bfU^{(t)};\bfX_{\ns[t](v)})}{\partial \bfw_k} \Big|_{\bfw_k=\bfw_k^{(t)}} = \bfp_+.
\end{equation}
For $v\in\Omega_-$ and a lucky neuron $\bfw_k^{(t)}$, we have 
\begin{equation}
    \mathcal{M}^{(t)}(v;\bfw_k^{(t)}) \in \{\bfx_n \}_{n\in\ns[t](v)}\bigcup \{\bfzero\},   
\end{equation}
and the gradient can be represented as
\begin{equation}\label{eqn: lemma1_1_-}
    \frac{\partial g(\bfW^{(t)},\bfU^{(t)};\bfX_{\ns[t](v)})}{\partial \bfw_k}\Big|_{\bfw_k=\bfw_k^{(t)}} = \mathcal{M}^{(t)}(v;\bfw_k^{(t)}).
\end{equation}
Because the neighbors of node $v$ with negative label do not contain $\bfp_+$, \eqref{eqn: lemma1_1_-} cannot be $\bfp_+$. In addition, $\bfp_+$ is orthogonal to $\{\bfx_n \}_{n\in\ns[t](v)} \bigcup \{\bfzero\}$. Then, we have 
\begin{equation}\label{eqn: lemma1_1_-1}
    \Big\langle \bfp_+, \frac{\partial g(\bfW,\bfU;\bfX_{\ns[t](v)})}{\partial \bfw_k}\Big|_{\bfw_k=\bfw_k^{(t)}} \Big\rangle = 0.
\end{equation}
Combining \eqref{eqn: lemma1_1_+}, \eqref{eqn: lemma1_1_-} and \eqref{eqn: lemma1_1_-1}, we have 
\begin{equation}
\begin{split}
    \vm{\bfw_k^{(t+1)}}{\bfp_+} 
    =& \vm{\bfw_k^{(t)}}{\bfp_+}  +\eta\cdot \vm{~\mathbb{E}_{v\in \Omega_+}\mathcal{M}^{(t)}(v;\bfw_k^{(t)}) - \mathbb{E}_{v\in \Omega_-}\mathcal{M}^{(t)}(v;\bfw_k^{(t)})}{~\bfp_+}\\
     =&\vm{\bfw_k^{(t)}}{\bfp_+}  +\eta\cdot \vm{~\mathbb{E}_{v\in \Omega_+}\mathcal{M}^{(t)}(v;\bfw_k^{(t)})}{~\bfp_+}\\
     =&\vm{\bfw_k^{(t)}}{\bfp_+}  +\eta\cdot \vm{~\mathbb{E}_{v\in \Omega_+}\mathcal{M}^{(t)}(v;\bfw_k^{(t)})}{~\bfp_+}\\
     \ge & \vm{\bfw_k^{(t)}}{\bfp_+} + \eta \|\bfp_+\|_2^2.
\end{split}
\end{equation}
For any $\bfz \in \{\bfx_n\}_{n\in\mathcal{N}(v)}$, we will prove the following equation by mathematical induction:
\begin{equation}\label{lemma1:1_1_1}
    -\eta\le  \vm{\bfw_k^{(t+1)}}{\bfz} \le \vm{\bfw_k^{(t)}}{\bfz}.
\end{equation}  
It is clear that \eqref{lemma1:1_1_1} holds when $t=0$. Suppose \eqref{lemma1:1_1_1} holds for $t$. When $\vm{\bfw_k^{(t+1)}}{\bfz}\le0$, we have
\begin{equation}
    \mathcal{M}(v;\bfw_k^{(t)}) \neq \bfz \quad  \text{for any} \quad v \in \{v\mid y_v =-1\}. 
\end{equation}
When $\vm{\bfw_k^{(t+1)}}{\bfz}>0$, we have 
\begin{equation}
    \begin{split}
        \vm{\bfw_k^{(t+1)}}{\bfz} 
    =& \vm{\bfw_k^{(t)}}{\bfz}  + \eta\cdot \vm{\mathbb{E}_{v \in \Omega_+}\mathcal{M}^{(t)}(v;\bfw_k^{(t)}) - \mathbb{E}_{v \in \Omega_-}\mathcal{M}^{(t)}(v;\bfw_k^{(t)})}{\bfz}\\
    =& \vm{\bfw_k^{(t)}}{\bfz}  - \eta\cdot \vm{\mathbb{E}_{v \in \Omega_-}\mathcal{M}^{(t)}(v;\bfw_k^{(t)})}{\bfz}\\
    \le & \vm{\bfw_k^{(t)}}{\bfz},
    \end{split}
\end{equation}
and 
\begin{equation}
    \begin{split}
        -\vm{\bfw_k^{(t+1)}}{\bfz} 
    =& -\vm{\bfw_k^{(t)}}{\bfz}  - \eta\cdot \vm{\mathbb{E}_{v \in \Omega_+}\mathcal{M}^{(t)}(v;\bfw_k^{(t)}) - \mathbb{E}_{v \in \Omega_-}\mathcal{M}^{(t)}(v;\bfw_k^{(t)})}{\bfz}\\
    =& -\vm{\bfw_k^{(t)}}{\bfz}  + \eta\cdot \vm{\mathbb{E}_{v \in \Omega_-}\mathcal{M}^{(t)}(v;\bfw_k^{(t)})}{\bfz}\\
    \le & \eta.
    \end{split}
\end{equation}
Therefore, \eqref{lemma1:1_1_1} holds for all $t\ge0$ by mathematical induction. 
\end{proof}


\subsection{Proof of Lemma \ref{Lemma: update_unlucky_neuron}}
\begin{proof}[Proof of Lemma \ref{Lemma: update_unlucky_neuron}]
    From \eqref{eqn: update_g_2}, we have
    \begin{equation}
    \begin{split}
    \vm{\bfw_k^{(t+1)}}{\bfp_+} 
    =& \vm{\bfw_k^{(t)}}{\bfp_+}  + \eta\cdot \vm{\mathbb{E}_{v\in\Omega_+}\mathcal{M}^{(t)}(v;\bfw_k^{(t)}) - \mathbb{E}_{v\in\Omega_-} \mathcal{M}^{(t)}(v;\bfw_k^{(t)})}{~\bfp_+}\\
    =& \vm{\bfw_k^{(t)}}{\bfp_+}  + \eta\cdot \vm{\mathbb{E}_{v\in\Omega_+}\mathcal{M}^{(t)}(v;\bfw_k^{(t)})}{~\bfp_+}\\
    \le & \vm{\bfw_k^{(t)}}{\bfp_+}.
    \end{split}
\end{equation}
Next, we will bound $\vm{\bfw_k^{(t)}}{\bfp_-}$. 
Similar to the proof of \eqref{lemma1:1_1_1}, we will prove the following equation by mathematical induction:
\begin{equation}\label{lemma2:1_1_1}
    -\eta \le \vm{\bfw_k^{(t+1)}}{\bfp_-} \le \vm{\bfw_k^{(t)}}{\bfp_-}.
\end{equation}  
It is clear that \eqref{lemma2:1_1_1} holds when $t=0$. Suppose \eqref{lemma2:1_1_1} holds for $t$. When $\vm{\bfw_k^{(t+1)}}{\bfp_-}\le0$, we have
\begin{equation}
    \mathcal{M}^{(t)}(v;\bfw_k^{(t)}) \neq \bfp_- \quad  \text{for any} \quad v \in \Omega_-. 
\end{equation}
Therefore, from \eqref{eqn: update_g_2}, we have
\begin{equation}
    \begin{split}
    \vm{\bfw_k^{(t+1)}}{\bfp_-} 
    =& \vm{\bfw_k^{(t)}}{\bfp_-}  + \eta\cdot \vm{\mathbb{E}_{v\in \Omega_+}\mathcal{M}^{(t)}(v;\bfw_k^{(t)}) - \mathbb{E}_{v\in\Omega_-}\mathcal{M}(v;\bfw_k^{(t)})}{~\bfp_-}\\
    = & \vm{\bfw_k^{(t)}}{~\bfp_-}.
    \end{split}
\end{equation}
When $\vm{\bfw_k^{(t+1)}}{\bfp_-}>0$, we have 
\begin{equation}
    \begin{split}
        \vm{\bfw_k^{(t+1)}}{\bfp_-} 
    =& \vm{ \bfw_k^{(t)} }{ \bfp_- }  
    + \eta\cdot \vm{ \mathbb{E}_{v \in \Omega_+} \mathcal{M}^{(t)} (v;\bfw_k^{(t)} ) - \mathbb{E}_{ v \in \Omega_-} \mathcal{M}^{(t)} (v;\bfw_k^{(t)}) }{~\bfp_-}
    \\
    =& 
    \vm{ \bfw_k^{(t)} }{ \bfp_- }  - \eta \cdot 
    \vm{ \mathbb{E}_{ v \in \Omega_- } \mathcal{M}^{(t)}( v;\Omega_-) }{~\bfp_-}
    \\
    \le & \vm{ \bfw_k^{(t)} }{ \bfp_- },
    \end{split}
\end{equation}
and 
\begin{equation}
    \begin{split}
        -\vm{\bfw_k^{(t+1)}}{\bfp_-} 
    =& -\vm{\bfw_k^{(t)}}{\bfp_-}  - \eta\cdot \vm{\mathbb{E}_{ v \in \Omega_+}\mathcal{M}^{(t)}(v;\bfw^{(t)}_k) - \mathbb{E}_{v \in \Omega_-}\mathcal{M}^{(t)}(v;\bfw^{(t)}_k)}{~\bfp_-}\\
    =& -\vm{\bfw_k^{(t)}}{\bfp_-}  + \eta\cdot \vm{\mathbb{E}_{v\in\Omega_-}\mathcal{M}^{}(t)(v;\bfw^{(t)})}{~\bfp_-}\\
    \le & \eta.
    \end{split}
\end{equation}
Therefore, \eqref{lemma2:1_1_1} holds for all $t\ge0$ by mathematical induction. 

To bound $|\vm{\bfw_k^{(t+1)}}{\bfz} - \vm{\bfw_k^{(t)}}{\bfz}|$ for any fixed $\bfz \in \mathcal{P}_s$, we maintain the subsets $\mathcal{S}_k(t) \subseteq \Omega_-$ such that $\mathcal{S}_k(t) = \{v\in \Omega_- \mid \mathcal{M}^{(t)}(v;\bfw_k^{(t)})= \bfp_- \}$. 

First,  When $\mathcal{S}_k(t)=\emptyset$, it is easy to verify that 
\begin{equation}\label{eqn:lemma2_t2}
    \vm{\bfw_k^{(t+1)}}{\bfp_-} = \vm{\bfw_k^{(t)}}{\bfp_-}.
\end{equation}
Therefore, $\mathcal{S}_k(t+1)=\emptyset$ and $\mathcal{S}_k(t')=\emptyset$ for all $t'\ge t$. 

Second, when $\mathcal{S}_k(t)\neq\emptyset$, then we have \begin{equation}
    \vm{\bfw_k^{(t+1)}}{\bfp_-} = \vm{\bfw_k^{(t)}}{\bfp_-} - \eta \cdot \frac{|\mathcal{S}_k(t)|}{|\Omega_-|} \|\bfp_-\|^2.
\end{equation}
Note that if $\vm{\bfw_k^{(t)}}{\bfp_-}<0$, then $\mathcal{S}_k(t)$ must be an empty set. Therefore, after at most $t_0 = \frac{\|\bfw_k^{(0)}\|_2}{\eta}$ number of iterations, $\mathcal{S}_k(t_0) =\emptyset$, and $\mathcal{S}_k(t) =\emptyset$ with $t\ge t_0$ from \eqref{eqn:lemma2_t2}.  

Next, for some large $t_0$ and any $v\in\mathcal{V}$, we define a mapping $\mathcal{F}: \mathcal{V}\longrightarrow \mathbb{R}^{rd}$ such that 
\begin{equation}
    \mathcal{F}(v) = \begin{bmatrix} \bfz_{v_1}^\top & \bfz_{v_2}^\top & \cdots & \bfz_{v_r}^\top \end{bmatrix}^\top.
\end{equation}
From \eqref{eqn: update_g_2}, we have 
\begin{equation}
    \vm{\bfw_k^{(t+1)}}{\bfz} - \vm{\bfw_k^{(t)}}{\bfz}
    = \eta\cdot \mathbb{E}_{v\in \mathcal{V} }\vm{ y_v\mathcal{M}^{(t)}(v;\bfw_k^{(t)})}{\bfz},
\end{equation}
where $\{v_1, \cdots, v_r \} = \ns[t](v)$ and 
\begin{equation}
    \begin{cases}
        \bfz_{v_i} = \bfx_{v_i}, \quad \text{if $\bfx_{v_1}\neq \bfp_+$ or $\bfp_-$}\\
        \bfz_{v_i} = \bfzero, \quad \text{if $\bfx_{v_1}= \bfp_+$ or $\bfp_-$}
    \end{cases}.
\end{equation}

When $y=1$, we have 
\begin{equation}\label{eqn:lemma2_1}
    \vm{\mathcal{M}(\bfx)}{\bfz}=
    \begin{cases}
        \vm{\mathcal{M}^{(t)}(\mathcal{F}(v))}{\bfz}, \quad \text{if} \quad \mathcal{M}^{(t)}(\mathcal{F}(v)) \neq \bfp_+ \\
         0 \le \vm{\mathcal{M}^{(t)}(\mathcal{F}(v))}{\bfz}, \quad \text{if} \quad \mathcal{M}^{(t)}(\mathcal{F}(v)) = \bfp_+
    \end{cases}.
\end{equation}
When $y=-1$ and $t\ge t_0$, recall that $\mathcal{S}_k(t) = \mathcal{D}_-$, then we have
\begin{equation}\label{eqn:lemma2_2}
    \vm{\mathcal{M}(\bfx)}{\bfz}=\vm{\mathcal{M}(\mathcal{F}(\bfx))}{\bfz}.
\end{equation}
Combining \eqref{eqn:lemma2_1} and \eqref{eqn:lemma2_2}, we have
\begin{equation}
\begin{split}
    \vm{\bfw_k^{(t+1)}}{\bfz} - \vm{\bfw_k^{(t)}}{\bfz}
    \le& \eta\cdot \mathbb{E}_{ v \in \mathcal{V} } \big[y \cdot \vm{ \mathcal{M}(\mathcal{F}(v)) }{\bfz}\big].
    % \le & \eta\cdot \mathbb{E}_{y}y\cdot \mathbb{E}_{\bfx}\vm{\mathcal{M}(\mathcal{F}(\bfx))}{\bfz}\\
    % \lesssim & \eta \cdot \sqrt{\frac{d\log q}{N}} \cdot \frac{M}{L}.
\end{split}
\end{equation}
It is clear to see that $y$ and $\mathcal{F}(v)$ are independent with each other, then we have
\begin{equation}
\begin{split}
    \vm{\bfw_k^{(t+1)}}{\bfz} - \vm{\bfw_k^{(t)}}{\bfz}
    \le & \eta \cdot \mathbb{E}_{v\in\mathcal{V}} y_v\cdot \mathbb{E}_{v}\vm{\mathcal{M}(\mathcal{F}(v))}{\bfz}.\\
    % \lesssim & \eta \cdot \sqrt{\frac{d\log q}{N}} \cdot \frac{M}{L}.
\end{split}
\end{equation}
Recall that Prob($y=1$) = $\frac{1}{2}$ and Prob($y=-1$) = $\frac{1}{2}$. 
By Hoeffding bound, we have 
\begin{equation}\label{eqn: lemma3_temp_1}
    \frac{1}{|\Omega|}\Big( \sum_{ v\in \Omega_+} y_v + \sum_{ v\in \Omega_-} y_v \Big) \le \sqrt{ \frac{ d \log q }{ N } }
\end{equation}
with probability at least $1 - q^{-d}$.

% Let we define an indicator $I_{\bfx}$ such that 
% \begin{equation}
%     I_{\bfx} = 
%     \begin{cases}
%         1, \quad \text{if $\bfx$ contains $\bfz$}\\
%         0, \quad \text{if $\bfx$ does not contain $\bfz$}\\
%     \end{cases}.
% \end{equation}
% It is easy to verify that $I_{\bfx}$ belongs to Bernoulli distribution. The probability of value $1$ (mean of $I_{\bfx}$) is calculated as 
% \begin{equation}\label{defi: p_0}
% \begin{split}
%     P_0 = & \sum_{r=0}^M \Big[1-(1-\frac{1}{L})^r\Big] \text{Prob}(r)\\
%         = & 1 - \sum_{r=0}^M (1-\frac{1}{L})^r \binom{M}{r} \beta^r(1-\beta)^{M-r}\\
%         = & 1 - \sum_{r=0}^M \binom{M}{r} \Big(\beta\big(1-\frac{1}{L}\big)\Big)^r(1-\beta)^{M-r}\\
%         = & 1- (1-\beta + \beta -\frac{\beta}{L})^M\\
%         = & 1- \Big(1 - \frac{\beta}{L}\Big)^M.
% \end{split}     
% \end{equation}
% Then, 
% by Hoeffding bound, we have 
% \begin{equation}
%     \frac{1}{|\mathcal{D}|}\sum_{\bfx\in\mathcal{D}} I_{\bfx} \le P_0 + \sqrt{\frac{C\log q}{N}}.
% \end{equation}
% Hence, we have 
% \begin{equation}\label{eqn: lemma3_temp_2}
% \begin{split}
%     \mathbb{E}_{\bfx}\vm{\mathcal{M}(\mathcal{F}(\bfx))}{\bfz}
%     =& \mathbb{E}_{\bfx}\vm{\mathcal{M}(\mathcal{F}(\bfx))}{\bfz} \cdot I_{\bfx}\\
%     \le& \|\bfz\|^2 \mathbb{E}_{\bfx} I_{\bfx}\\
%     \le& \bigg(  P_0 + \sqrt{\frac{C\log q}{N}} \bigg)\|\bfz\|^2.
% \end{split}
% \end{equation}
% From \eqref{eqn: lemma3_temp_1} and \eqref{eqn: lemma3_temp_2}, 
% we have
% \begin{equation}
% \begin{split}
%     \vm{\bfw_k^{(t+1)}}{\bfz} - \vm{\bfw_k^{(t)}}{\bfz}
%     \le & \eta\cdot \mathbb{E}_{y}y\cdot \mathbb{E}_{\bfx}\vm{\mathcal{M}(\mathcal{F}(\bfx))}{\bfz}\\
%     \le & \eta\cdot\Big(P_0\sqrt{\frac{C\log q}{N}} + \frac{C\log q}{N}\Big)\cdot\|\bfz\|^2.
% \end{split}
% \end{equation}
\end{proof}

\subsection{Proof of Lemma \ref{Lemma: number_of_lucky_filter}}
\begin{proof}[Proof of Lemma \ref{Lemma: number_of_lucky_filter}]
    For any $k\in\mathcal{U}(0)$, we have 
    \begin{equation}\label{eqn:lemma3:1}
        \vm{\bfw_k^{(0)}}{\bfp_+} \ge \vm{\bfw_k^{(0)}}{\bfz}
    \end{equation}
    for any $\bfz\in\mathcal{P}/\bfp_+$ by the definition of \textit{lucky filter} in \eqref{defi:lucky_filter}.
    
    Next, from Lemma \ref{Lemma: update_lucky_neuron}, we have 
    \begin{equation}\label{eqn:lemma3:2}
        \begin{gathered}
            \vm{\bfw_k^{(t)}}{\bfp_+} 
            \ge \vm{\bfw_k^{(0)}}{\bfp_+}, \quad \text{and} \quad
            \vm{\bfw_k^{(t)}}{\bfz} 
            \le \vm{\bfw_k^{(0)}}{\bfz}.
        \end{gathered}
    \end{equation}
    Combining \eqref{eqn:lemma3:1} and \eqref{eqn:lemma3:2}, we have 
    \begin{equation}
        \vm{\bfw_k^{(t)}}{\bfp_+}\ge \vm{\bfw_k^{(t)}}{\bfz}.
    \end{equation}
    Therefore, we have $k\in \mathcal{U}(t)$ and
    \begin{equation}
        \mathcal{U}(0) \subseteq \mathcal{U}(t).
    \end{equation}
\end{proof}


\section{Extension to multi-class classification}\label{sec: multi-class}
Consider the classification problem with four classes, we use the label $\bfy\in\{+1,-1\}^{2}$ to denote the corresponding class. Similarly to the setup in Section \ref{sec: problem_formulation}, there are four orthogonal discriminative patterns, namely $\bfp_1, \bfp_2, \bfp_3, \bfp_4$. In the first layer (hidden layer), we have $K$ neurons with weights $\bfw_k\in\mathbb{R}^d$. 
In the second layer (linear layer), the weights are denoted as $v_k\in\mathbb{R}^2$ for the $k$-th neuron. Let $\bfW\in\mathbb{R}^{d \times K}$ and  $\bfV\in\mathbb{R}^{2\times K}$ be the collections of $\bfw_k$'s and $\bfv_k$'s, respectively. Then, the output of the graph neural network, denoted as $\bfg\in\mathbb{R}^2$, is calculated as   
\begin{equation}\label{eqn: useless1}
    \bfg(\bfW,\bfV;\bfX_{\mathcal{N}(v)}) = \frac{1}{K}\sum_{k=1}^K \bfv_k \cdot\text{AGG}(\bfX_{\mathcal{N}(v)},\bfw_k).
\end{equation}
Then, the label generated by the graph neural network is written as
\begin{equation}
    \bfy_{\text{est}} = \text{sign}(\bfg).
\end{equation}


\begin{figure}[h]
    \centering
    \includegraphics[width=0.7\linewidth]{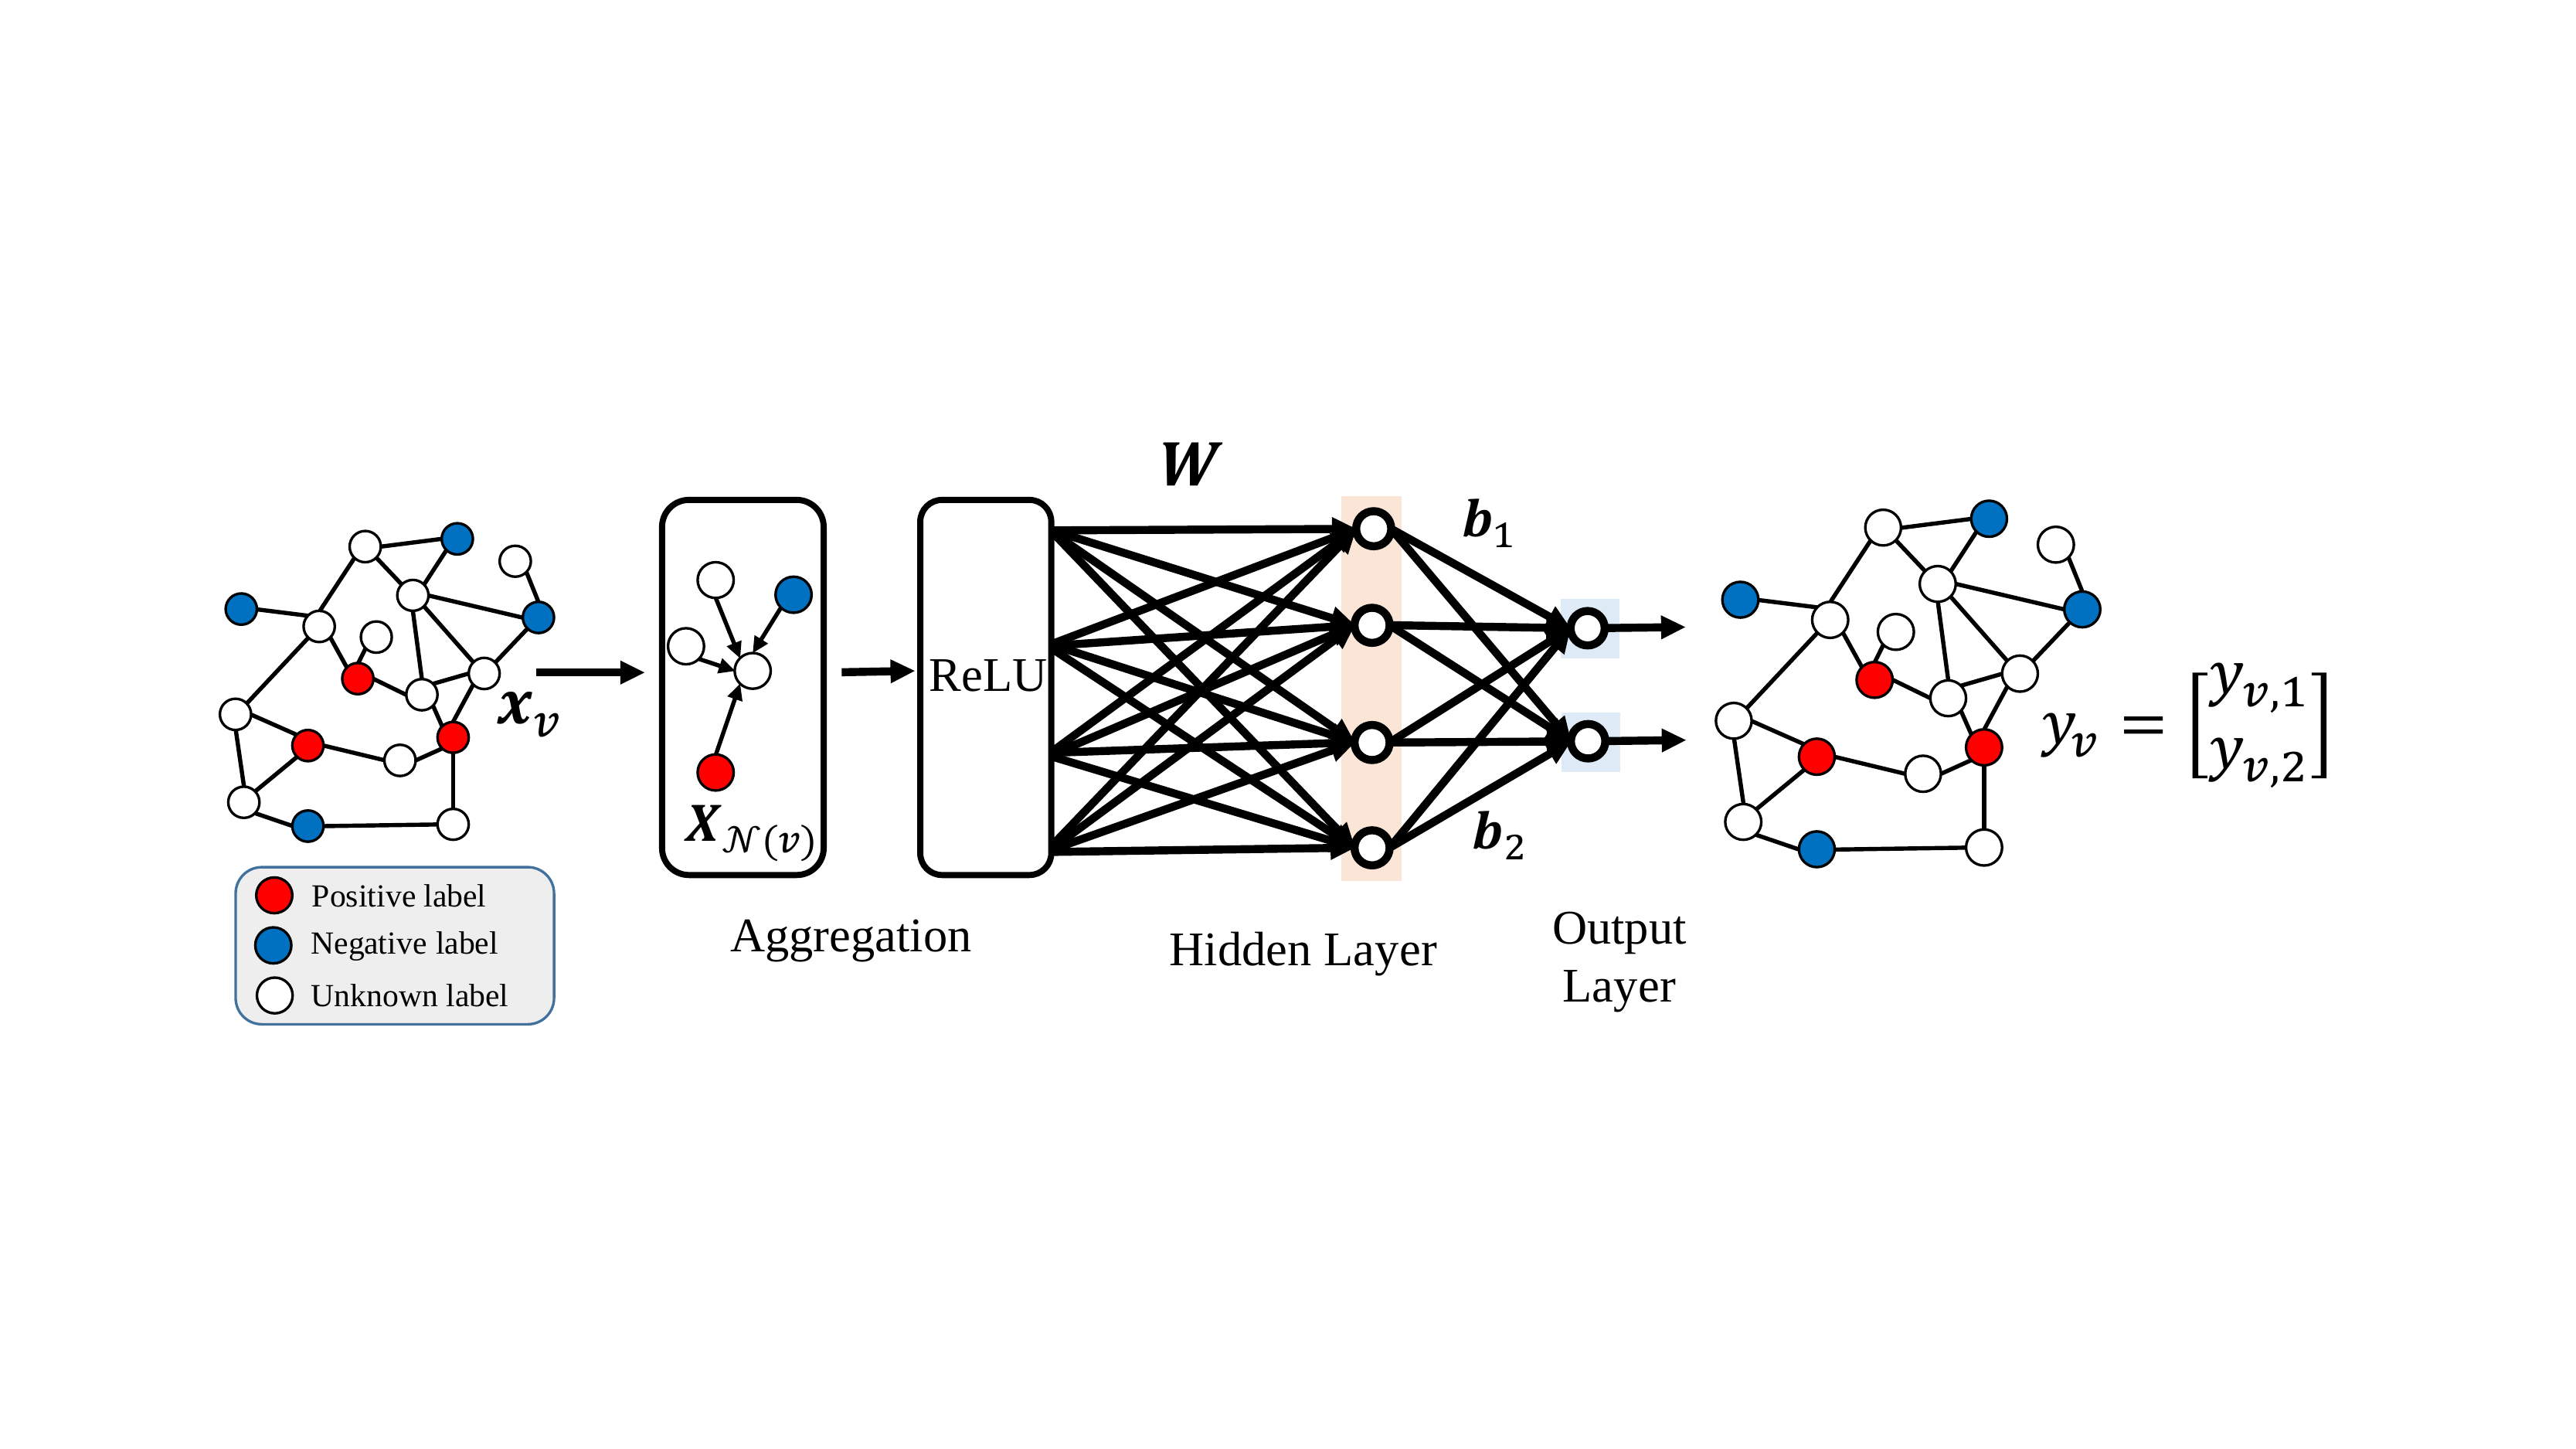}
    \caption{Illustration of graph neural network learning for multi-class classification}
    \label{fig:sage_multi}
\end{figure}

Given the set of data $\Omega$, we divide them into four groups as 
\begin{equation}
    \begin{gathered}
        \Omega_1 = \{ (\bfx , \bfy) \mid \bfy = ( 1 , 1 ) \},\\
        \Omega_2 = \{ (\bfx , \bfy) \mid \bfy = ( 1 , -1 ) \},\\
        \Omega_3 = \{ (\bfx , \bfy) \mid \bfy = ( -1 , 1 ) \},\\
        \text{and} \quad \Omega_4 = \{ (\bfx , \bfy) \mid \bfy = ( -1 , -1 ) \}.
    \end{gathered}
\end{equation}
The corresponding loss function in \eqref{eqn: ERF} need to be revised as 
\begin{equation}
\begin{split}
    \hat{f}_{\Omega}(\bfW,\bfU) 
    = &\sum_{i=1}^4-\frac{1}{|\Omega_i|}\sum_{ v \in \Omega_i } \bfy_v^\top \bfg\big(\bfW,\bfV;\bfX_{\mathcal{N}(v)} \big)\\
\end{split}
\end{equation}

Then, we initialize the weights of $\bfv_k$ as $(1,1), (1,-1), (-1,1),$ and $(-1,-1)$ equally. Next, we divide the weights $\bfw_k$ into four groups based on the value of $\bfv_k$, such that
\begin{equation}
    \begin{gathered}
        \mathcal{W}_1 = \{ k \mid \bfv_k = (1,1)\},\\
        \mathcal{W}_2 = \{ k \mid \bfv_k = (1,-1)\},\\
        \mathcal{W}_3 = \{ k \mid \bfv_k = (-1,1)\},\\
        \text{and} \quad \mathcal{W}_4 = \{ k \mid \bfv_k = (-1,-1)\}.\\
    \end{gathered}
\end{equation}
Hence, for any $k$ in $\mathcal{W}_1$, we have 
\begin{equation}\label{eqn: w1}
    \frac{\partial f}{\partial \bfw} 
    = - \frac{1}{|\Omega|} \sum_{v \in \Omega} y_{v,1} \cdot  \frac{\partial g_1}{\partial \bfw} - y_{v,2}   \cdot  \frac{\partial g_2}{\partial \bfw}.
\end{equation}
When $x\in \Omega_1$, we have 
\begin{equation}\label{eqn: w11}
    y_{v,1} \cdot  \frac{\partial g_1}{\partial \bfw} - y_{v,2}   \cdot  \frac{\partial g_2}{\partial \bfw}
    = -2\phi^{\prime}(\bfw^\top \bfx)\cdot \bfx.
\end{equation}
When $x\in \Omega_2$, we have 
\begin{equation}
    y_{v,1} \cdot  \frac{\partial g_1}{\partial \bfw} - y_{v,2}   \cdot  \frac{\partial g_2}{\partial \bfw}
    = 0.
\end{equation}
When $x\in \Omega_3$, we have
\begin{equation}
    y_{v,1} \cdot  \frac{\partial g_1}{\partial \bfw} - y_{v,2}   \cdot  \frac{\partial g_2}{\partial \bfw}
    = 0.
\end{equation}
When $x\in \Omega_4$, we have 
\begin{equation}
    y_{v,1} \cdot  \frac{\partial g_1}{\partial \bfw} - y_{v,2}   \cdot  \frac{\partial g_2}{\partial \bfw}
    = 2\phi^{\prime}(\bfw^\top \bfx)\cdot \bfx.
\end{equation}
By following similar analysis in \textcolor{red}{($\cdots$)}, for any $k\in \mathcal{W}_1$, we have 
\begin{equation}\label{eqn: w}
\begin{gathered}
    \vm{\bfw^{(t+1)} - \bfw^{(t)}}{\bfp_1} = 2\|\bfp_1 \|_2^2,\\
    \vm{\bfw^{(t+1)} - \bfw^{(t)}}{\bfp_2} = 0,\\
    \vm{\bfw^{(t+1)} - \bfw^{(t)}}{\bfp_3} = 0,\\
    \text{and} \quad \vm{\bfw^{(t+1)} - \bfw^{(t)}}{\bfp_4} \le 0.
\end{gathered}
\end{equation}
Therefore, for any $k\in \mathcal{W}_1$, the weights $\bfw_k^{(t)}$ will update along the direction of $\bfp_1$. By following the steps in \eqref{eqn: w1} to \eqref{eqn: w}, we can derive that $\bfw_k^{(t)}$ will  update purely along the direction of $\bfp_i$ for any $k\in\mathcal{W}_i$.
